# Supplementary material for: Equivariant Similarity for Vision-Language Foundation Models
Source: arXiv:2303.14465 source file (2023-10-09)
Supplement: Supplementary file 1 [file supp_kubric.tex]

\begin{table*}[t]
\tablestyle{5pt}{1.5} 
\begin{tabular}{cccccc}
\shline
 & Template & object & verb & location & subject \\ \hline
 \rule{0pt}{30pt}
\multirow{2}{*}{Location} & \multirow{2}{1in}{The $\langle$\textit{object}$\rangle$ $\langle$\textit{verb}$\rangle$ $\langle$\textit{location}$\rangle$ the $\langle$\textit{subject}$\rangle$} & \multirow{6}{2in}{green turtle toy, white animal dog toy, black power pressure cooker, great white shark model, white ramekin porcelain, pink damask bath towel, white porcelain teapot, grey elephant toy, bald eagle toy, brown bull, blue gloves, brown hat, white gaming mouse, black keyboard, black boot, white gift box with red straps, red scissors, vintage metal alarm clock, black frypan, stainless steel milk frother, red coffee mug, purple doll house wooden sofa, black sneaker, white canvas shoe, black laptop, black and red gameboy, blue and black backpack, red high heel, stainless steel toaster, white drug bottle, fabric basket, school bus toy, black and yellow hammer, green doll house wooden refrigerator} & \multirow{4}{1in}{is, is located, is placed} & \multirow{4}{*}{} & \multirow{6}{*}{} \\
 &  &  &  &  &  \\ \cline{1-2}
\multirow{2}{*}{Attribute} & \multirow{2}{*}{} &  &  &  &  \\
 &  &  &  &  &  \\ \cline{1-2}
\multirow{2}{*}{Counting} & \multirow{2}{*}{} &  &  &  &  \\
 &  &  &  &  &  \\ \hline
\end{tabular}
\end{table*}
